# Supplementary material for: Font Representation Learning via Paired-glyph Matching
Source: arXiv:2211.10967 source file (2022-11-20)
Supplement: Supplementary file 1 [file supplementary.tex]

For training, and testing we used the following 22 joints: Root, Spine, Spine1, Spine2, Neck, Head, LeftUpLeg, LeftLeg, LeftFoot, LeftToeBase, RightUpLeg, RightLeg, RightFoot, RightToeBase, LeftShoulder, LeftArm, LeftForeArm, LeftHand, RightShoulder, RightArm, RightForeArm, and RightHand.

training 7명: (AJ, Big Vegas, Goblin Shareyko, Kaya, Malcolm, Peasant Man, and Warrok Kurniawan)
The target characters are Malcolm, Warrok W ...

\subsection{Implementation Details}
\label{Implementation}

\begin{itemize}
\item Network architectures
    \begin{itemize}
    \item Local 
    \item Global
    \item Discriminators
    \end{itemize}
\item Training details
    \begin{itemize}
    \item NKN과 마찬가지로 autoregress loss 를 사용했다. 
    \item Adam optimizer~\cite{kingma2014adam}
    \end{itemize}
\item tensorflow~\cite{abadi2016tensorflow}로 구현.
\item 코드 공개 하겠다.
\end{itemize}

Dataset preprocess: 
From NKN:
Each motion sequence is preprocessed by separating into local and global motion, similar to~\cite{holden2016deep}.
For local motion, we remove the global displacement (\ie, the motion of the root joint), and rotation around the axis vertical to the ground.
Global motion consists of the velocity of the root in the $x$, $y$, and $z$ directions, and an additional value representing the rotation around the axis perpendicular to the ground. 
, which is suitable for training than 3D joint positions~\cite{holden2016deep}.
