# Supplementary material for: Font Representation Learning via Paired-glyph Matching
Source: arXiv:2211.10967 source file (2022-11-20)
Supplement: Supplementary file 3 [file fig-supplementary_capitals_to_donovan_classes.tex]

\begin{figure*}[]\centering
\includegraphics[width=0.92\linewidth]{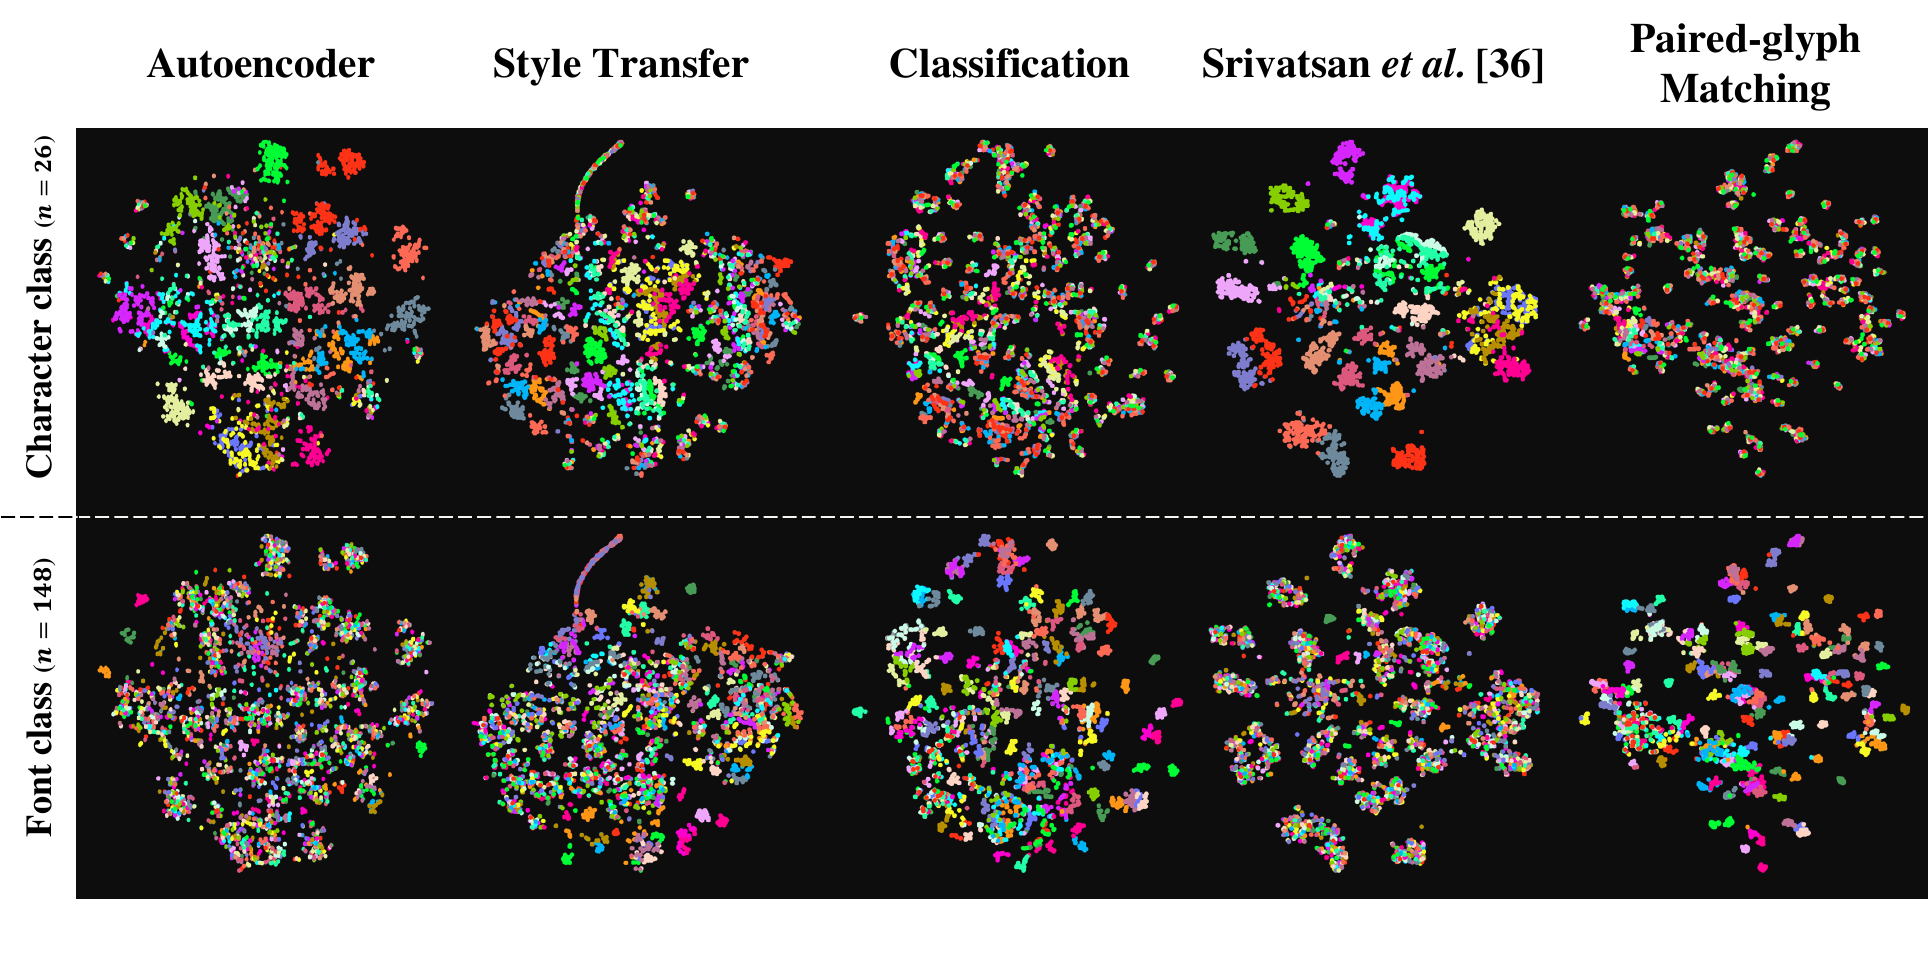}
\vspace*{-0.3cm}
\caption{Font latent space on the O'Donovan dataset annotated by font and character classes.
} 
% \Description{Font Embedding Methods with attributes}
\label{fig:supplementary_capitals_to_donovan_classes}
\vspace{-0.3cm}
\end{figure*}
