# Supplementary material for: Font Representation Learning via Paired-glyph Matching
Source: arXiv:2211.10967 source file (2022-11-20)
Supplement: Supplementary file 4 [file fig-supplementary_linear_evaluation_protocol.tex]

\begin{figure}
  \centering
  \includegraphics[width=0.5\linewidth]{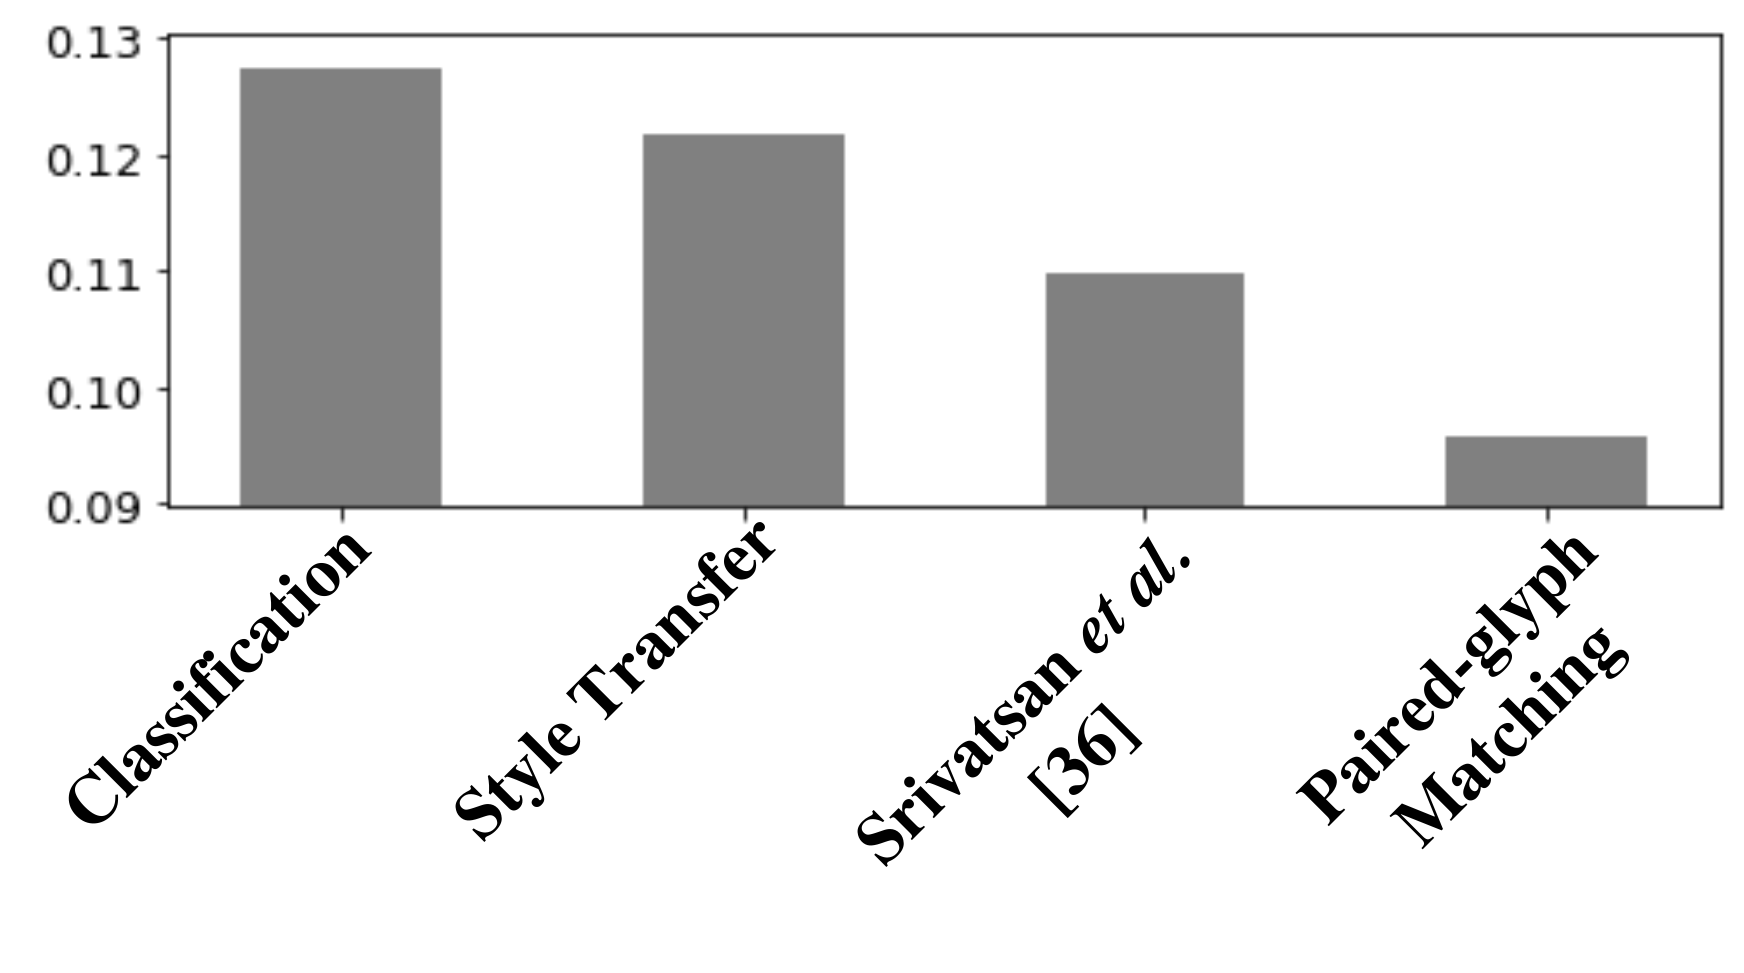}
  \vspace{-0.8cm}
  \caption{
  Font attribute prediction results from $\hat{f}$ of each method.
  }
%   \Description{Anatomy of typography.}
  \label{fig:supplementary-linear-evaluation-protocol}
\end{figure}
