# Supplementary material for: Font Representation Learning via Paired-glyph Matching
Source: arXiv:2211.10967 source file (2022-11-20)
Supplement: Supplementary file 5 [file fig-supplementary_loss_function.tex]

\begin{figure}[h]
  \centering
  \includegraphics[width=1.0\linewidth]{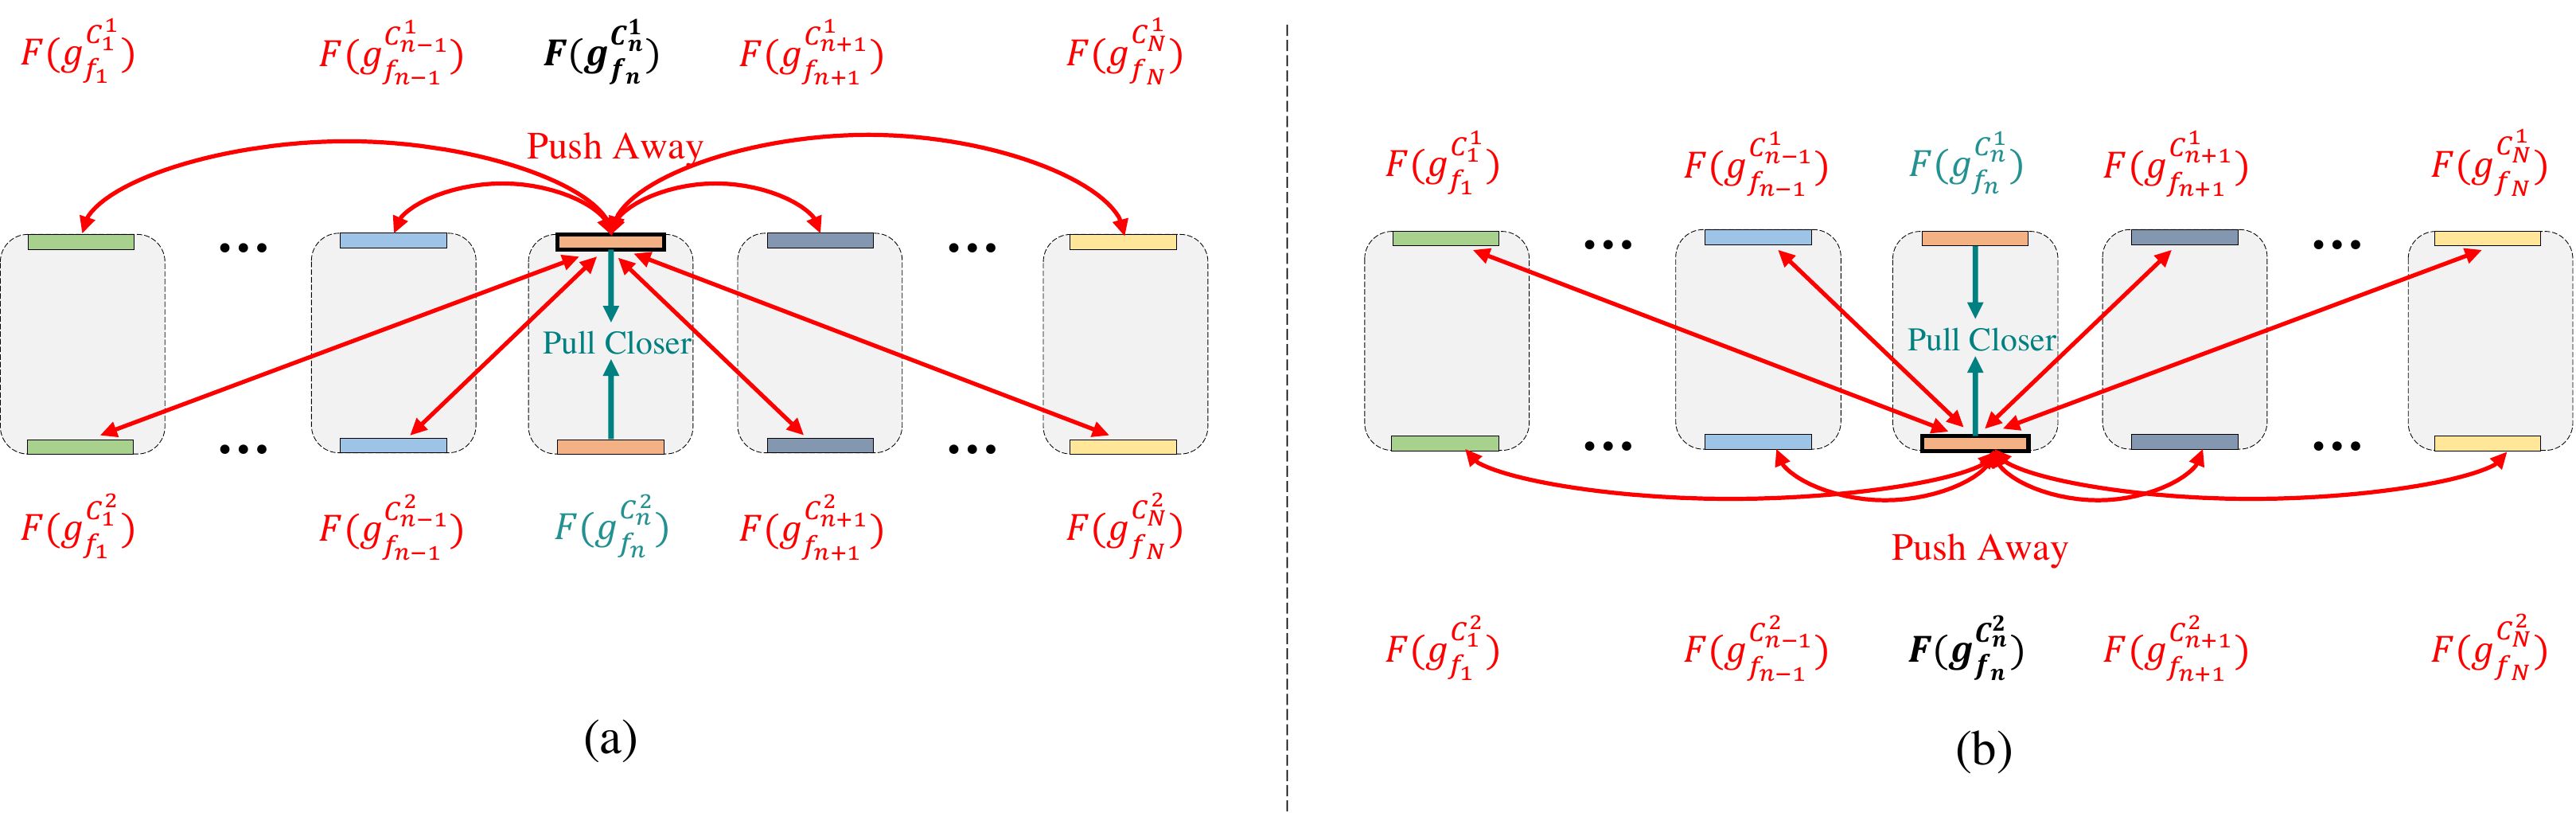}
  \caption{
  Detailed description on the loss function of {\it Paired-glyph Matching} learning.
  }
%   \Description{Detailed description on the loss function of {\it Paired-glyph Matching} learning. }
  \label{fig:supplementary_loss_fuction}
\end{figure}
